# Supplementary material for: Doomed to Re-Annotate, Forever: The ImageNet Story
Source: arXiv:2608.13783 source file (2026-08-13)
Supplement: Supplementary file 1 [file additional_sets.tex]

\begin{table}[t]
    \caption{Results on additional ImageNet test sets.}
    \label{tab:additional_sets_2}
    \small
    % \setlength{\tabcolsep}{3.8pt}
    \begin{tabular}{lrr rrr rrr rr}
        \toprule
        & & & \multicolumn{2}{c}{\cgpt}
            & \multicolumn{2}{c}{\sigliptwog}
            & \multicolumn{2}{c}{\effnetl} \\
        \cmidrule(lr){4-5}
        \cmidrule(lr){6-7}
        \cmidrule(lr){8-9}
        Dataset & \# Cls. & \# Imgs. & In1k & Subset
                                      & In1k & Subset
                                      & In1k & Subset \\
        \midrule
        ImageNetV2      & 1000 & 10{,}000 & 64.13 & 64.13 & 80.24 & 80.24 & 81.42 & 81.42 \\
        ImageNet-A      & 200  & 7{,}500  & 45.13 & 57.25 & 74.69 & 89.57 & 61.73 & 84.65 \\
        ImageNet-R      & 200  & 30{,}000 & 76.89 & 84.05 & 85.95 & 95.44 & 56.64 & 74.61 \\
        ImageNet-Sketch & 1000 & 50{,}889 & 55.15 & 55.15 & 77.00 & 77.00 & 48.03 & 48.03 \\
        ObjectNet       & 125  & 18{,}574 & 68.01 & 72.35 & 74.10 & 80.87 & 61.07 & 69.67 \\
        CounterAnimal   & 45   & 13{,}334 & 75.45 & 86.61 & 91.05 & 94.98 & 90.30 & 93.22 \\
        \bottomrule
    \end{tabular}
\end{table}
